# Supplementary material for: Accurate Neural Network Pruning Requires Rethinking Sparse Optimization
Source: arXiv:2308.02060 source file (2023-09-08)
Supplement: Supplementary file 1 [file appendix.tex]

\appendix

\tableofcontents
